# Supplementary material for: On Implementation of a Safer C Library, ISO/IEC TR 24731
Source: arXiv:0906.2512 source file (2009-07-27)
Supplement: Supplementary file 1 [file appendix.tex]

\appendix

\chapter{Something}

%\chapter{ChangeLog}

%\vspace{15pt}
%\hrule
%{\scriptsize \input{ChangLog}}
%\hrule
%\vspace{15pt}

% EOF
